# Supplementary material for: Unilateral Criticality and Phase Transition in the Cavity-Ising Model
Source: arXiv:2509.04391 ancillary file (2025-09-05)
Supplement: Supplementary file 1 [file supp.pdf]

# Supplementary material for "Unilateral Criticality and Phase Transition in the Cavity-Ising Model"

Zeyu Rao,<sup>1,2</sup> Xiaoshui Lin,<sup>1,2</sup> Xiwang Luo,<sup>1,2,3,4,\*</sup> Guangcan Guo,<sup>1,2,3,4</sup> Han Pu,<sup>5,†</sup> and Ming Gong<sup>1,2,3,4,‡</sup>

<sup>1</sup>Key Laboratory of Quantum Information, University of Science and Technology of China, Hefei 230026, China

<sup>2</sup>Anhui Province Key Laboratory of Quantum Network,  
University of Science and Technology of China, Hefei 230026, China

<sup>3</sup>Hefei National Laboratory, University of Science and Technology of China, Hefei 230088, China

<sup>4</sup>Synergetic Innovation Center of Quantum Information and Quantum Physics,  
University of Science and Technology of China, Hefei 230026, China

<sup>5</sup>Department of Physics and Astronomy, Rice University, Houston, Texas 77251-1892, USA

## CONTENTS

|                                                                 |    |
|-----------------------------------------------------------------|----|
| I. Three possible configurations                                | 1  |
| II. Competition between two order parameters: mean-field theory | 2  |
| III. Phase transition and scaling laws                          | 3  |
| A. Landau theory for phase transition                           | 3  |
| B. Critical exponent for second-order transition                | 4  |
| C. Critical exponent for tricritical transition                 | 4  |
| IV. Finite temperature effect                                   | 5  |
| V. Unilateral critical endpoint                                 | 7  |
| References                                                      | 14 |

## I. THREE POSSIBLE CONFIGURATIONS

For the model with one first-order transition and two second-order transitions, it is possible to have different types of intersections, which are shown in Fig. S1. In (a), we require that the two points, B and C, with physical meanings explained in the main text, merge at the same point, which requires some stringent conditions. This may happen in a lot of physical systems, yet it requires some special constraints, physically or mathematically, to ensure that these two points coincide at the same point. In (b) and (c), we can have two different points; however, in (b), it is possible

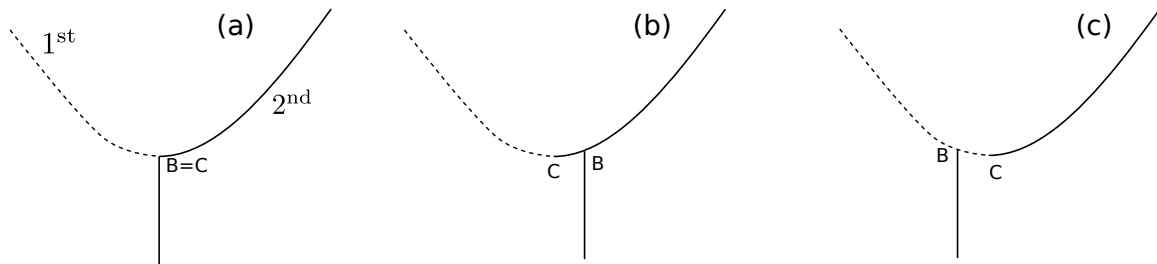

FIG. S1. Three possible cases for the intersection between one first-order and two second-order transition lines, with only three phases. 1<sup>st</sup> and 2<sup>nd</sup> refers to first and second-order transitions, respectively. In the main text, B and C are the intersections of transition lines.

\* xwluo@ustc.edu.cn

† hpu@rice.edu

‡ gongm@ustc.edu.cn

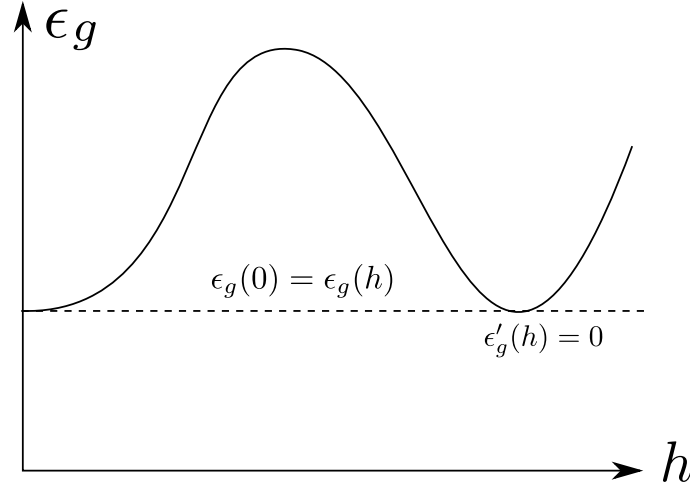

FIG. S2. The condition of first-order transition, which is used in the main text.

to have two successive spontaneous symmetry transitions, which is forbidden by a model with only  $\mathbb{Z}_2$  symmetry. As a result, we say that Fig. S1(c) is most natural to happen in a realistic system, which is indeed true in our model; see Fig. 1 in the main text. In this manuscript, the first-order transition can be obtained from the energy as a function of parameter  $h$ ; see Fig. S2 and see more details in the main text.

## II. COMPETITION BETWEEN TWO ORDER PARAMETERS: MEAN-FIELD THEORY

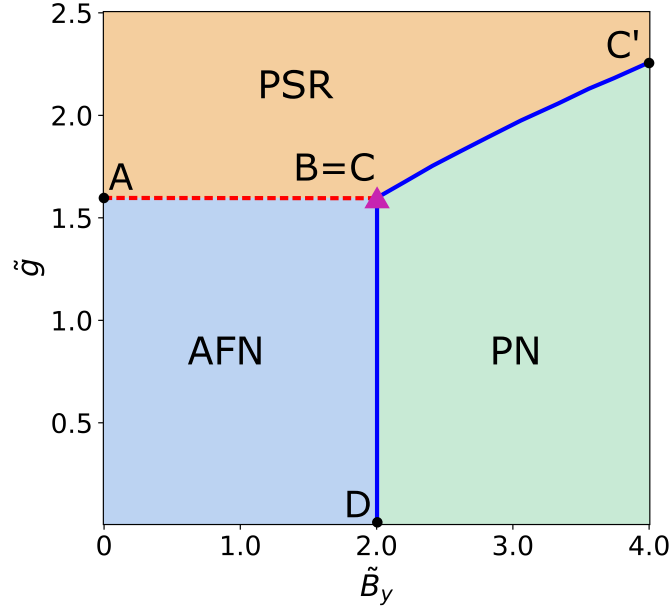

FIG. S3. The phase diagram obtained from the mean-field theory. The red dashed line is the first-order boundary, and the blue solid lines are the second-order lines. C is the intersection of three boundaries.

There is an intrinsic question that has not yet been fully understood: when we have defined two independent order parameters, why can the superradiant and antiferromagnetic order parameters not coexist, thus yielding only three different phases? Although the minimal universal free-energy description of the unilateral critical endpoint (UCEP) can naturally result in three phases, we try to address this problem using the mean-field theory. In this work, the

magnetic order can be defined as

$$m_s = \frac{1}{N} \sum_i (-1)^i \langle \sigma_i^z \rangle, \quad (\text{S1})$$

which is the staggered magnetic order. Thus, we can rewrite the  $\sigma_i^z$

$$\sigma_i^z = (-1)^i m_s + \underbrace{(\sigma_i^z - (-1)^i m_s)}_{\text{weak fluctuation}}. \quad (\text{S2})$$

Then it leads to

$$\begin{aligned} \sigma_i^z \sigma_{i+1}^z &= ((-1)^i m_s + (\sigma_i^z - (-1)^i m_s))((-1)^{i+1} m_s + (\sigma_{i+1}^z - (-1)^{i+1} m_s)) \\ &= m_s^2 - (-1)^i m_s \sigma_i^z - (-1)^{i+1} m_s \sigma_{i+1}^z, \end{aligned} \quad (\text{S3})$$

where we have ignored the fluctuation term  $(\sigma_i^z - (-1)^i m_s)(\sigma_{i+1}^z - (-1)^{i+1} m_s)$ , thus we have

$$J \sum_i \sigma_i^z \sigma_{i+1}^z = J N m_s^2 - 2 J m_s \sum_i (-1)^i \sigma_i^z. \quad (\text{S4})$$

With the above approximation, the Hamiltonian based on the mean-field approximation becomes

$$H_{\text{MF}} = N J \tilde{\gamma} \tilde{\alpha}^2 + J N m_s^2 + \tilde{\alpha} \sum_i \sigma_i^x - 2 J m_s \sum_i (-1)^i \sigma_i^z + B_y \sum_i \sigma_i^y, \quad (\text{S5})$$

where the  $\tilde{\gamma} = \frac{J\omega}{4g^2}$ ,  $\tilde{\alpha} = \frac{2g\alpha}{\sqrt{NJ}}$ . Now, all spins are decoupled in terms of mean-field approximation, we have the ground state energy density (at zero temperature,  $\epsilon_{\text{MF}} = E_{\text{MF}}/(NJ)$ )

$$\epsilon_{\text{MF}} = \tilde{\gamma} \tilde{\alpha}^2 + m_s^2 - \sqrt{\tilde{\alpha}^2 + 4m_s^2 + \tilde{B}_y^2}. \quad (\text{S6})$$

This energy contains two order parameters, and the competition between them yields the mean-field phase diagram in Fig. S3.

Comparing this phase diagram with the exact phase diagram in Fig. 1(a) in the main text, both of them contain a first-order transition line and two second-order transition lines. The major difference is that now the unilateral critical endpoint B and tricritical point C emerge to the same point (hence B=C), and the unilateral critical endpoint with one-sided criticality disappears. Besides, the phase boundary between AFN and PSR phases, which is a first-order transition, is a straight line, independent of  $\tilde{B}_y$ . A similar phase diagram can be found in Ref. [1] from the competition of two order parameters, yet in a totally different physical model. It should be noticed that in our model, we have two independent order parameters; thus, if we try to understand these results using mean-field theory, then in principle we should have four phases; however, the phase with  $\alpha \neq 0$  and  $m_s \neq 0$  will not appear in our phase diagram. The reason is that the following equation will have no solution

$$\frac{\partial \epsilon_{\text{MF}}}{\partial \alpha} = 0, \quad \frac{\partial \epsilon_{\text{MF}}}{\partial m_s} = 0, \quad (\text{S7})$$

when  $\alpha m_s \neq 0$ . In Ref. [1], the coexistence phase with two nonzero order parameters has been studied in a model with  $\mathbb{Z}_2 \times \mathbb{Z}_2$  symmetry. Therefore, based on mean-field theory, the superradiance and antiferromagnetism can not coexist. Another mechanism is that since our model only has  $\mathbb{Z}_2$  symmetry, it is impossible to have two successive spontaneous symmetry breakings.

### III. PHASE TRANSITION AND SCALING LAWS

#### A. Landau theory for phase transition

Let us consider the following model

$$V = \frac{\mu^2}{2} \Delta^2 + \lambda \Delta^4 + \kappa \Delta^6, \quad \Delta \in \mathbb{R}, \quad (\text{S8})$$

following the standard Landau theory of phase transition, where  $\kappa > 0$  to ensure stability. This paper automatically satisfy the  $\mathbb{Z}_2$  condition that

$$V(\Delta) = V(-\Delta). \quad (\text{S9})$$

We should have

1.  $\lambda > 0$ ,  $\mu^2 = 0$  for second-order transition;
2.  $\lambda < 0$  and  $\mu^2 = \lambda^2/(2\kappa)$  for first-order transition;
3.  $\lambda = 0$  and  $\mu^2 = 0$  for tricritical point.

The above energy  $V$  has a serious shortcoming that it is correct only when  $|\Delta|$  is small enough, while in the true condition, when  $|\Delta|$  is large, we can not make the above Taylor expansion anymore; see discussion in the main text. In this way, we should use the following criterion for the first-order transition as (see Fig. S2 with  $\Delta = h$ )

$$V(\Delta = 0) = V(\Delta), \quad V'(\Delta) = 0. \quad (\text{S10})$$

A picture of this mechanism using the energy of the Dicke-Ising model is shown in Fig. 1(b) in the main text for first-order transitions. It should be noticed that in the main text,  $V$  is denoted by  $\epsilon_g$ , which is the ground state energy at zero temperature, or  $V = f = F/N$  at finite temperature.

### B. Critical exponent for second-order transition

Let us first, to warm up, present the critical exponents for the second-order transition in the presence of some external parameter, say  $t$ , thus we have

$$V = t\Delta + \frac{\mu^2}{2}\Delta^2 + \lambda\Delta^4, \quad (\text{S11})$$

assume  $\lambda > 0$ , and  $t = A(g - g_c) \propto (g - g_c)$ , with  $g_c$  being the critical point, and  $(g - g_c)$  is the derivation from the critical point. We consider the following conditions.

1.  $\mu^2 = 0$  and  $t \neq 0$ . In this case, the minimal point has

$$t + 4\lambda\Delta^3 = 0, \quad \Delta = \left(-\frac{t}{4\lambda}\right)^{1/3}, \quad \epsilon_g \propto t^{4/3}. \quad (\text{S12})$$

2.  $\mu^2 > 0$ . In this case, we can ignore the quartic term and obtain

$$t + \mu^2\Delta = 0, \quad \Delta \propto t, \quad \epsilon_g \propto t^2. \quad (\text{S13})$$

3.  $\mu^2 < 0$  and  $t = 0$ . In this case, we have

$$\Delta = \sqrt{\frac{-\mu^2}{4\lambda}}, \quad \epsilon_g = -\frac{\mu^4}{16\lambda} \propto -\mu^4. \quad (\text{S14})$$

### C. Critical exponent for tricritical transition

With the above results, let us consider the tricritical point [2–11] with the following energy

$$V = t\Delta^2 + a\Delta^4 + \lambda\Delta^6. \quad (\text{S15})$$

The expressions for this energy can be found in the main text. We need  $\lambda > 0$  to ensure that  $V$  is bounded from below. Then, when  $a > 0$ , there will be a second-order phase transition while a first-order transition for  $a < 0$ . So the tricritical point is located at  $t = 0$ , and  $a = 0$ , as the intersection between second-order transition and first-order transition; see point C in the main text.

1.  $a = 0$  and  $t < 0$ . The minimal point gives

$$2t\Delta + 6\lambda\Delta^5 = 0, \quad \Delta^4 = -\frac{t}{3\lambda}, \quad \epsilon_g \propto -t^{3/2} \quad (\text{S16})$$

2.  $a < 0$  and  $t = 0$ , the minimal equation can be written as

$$4a\Delta^3 + 6\lambda\Delta^5 = 0, \quad \Delta^2 = -\frac{2a}{3\lambda}, \quad \epsilon_g \propto -a^3. \quad (\text{S17})$$

3.  $a = 0$  and  $t = 0$  with a small external field  $h$ . After introducing a linear external field,  $V$  becomes

$$V = \lambda\Delta^6 - h\Delta. \quad (\text{S18})$$

The minimal condition gives

$$6\lambda\Delta^5 - h = 0, \quad \Delta \propto h^{1/5}, \quad \epsilon_g \propto -h^{6/5}. \quad (\text{S19})$$

4.  $t > 0$  and  $a = 0$  with a small external field  $h$ .

$$V = t\Delta^2 + \lambda\Delta^6 - h\Delta, \quad (\text{S20})$$

and we have the following equation

$$2t\Delta + 6\lambda\Delta^5 - h = 0. \quad (\text{S21})$$

We can ignore the high-order term of  $\Delta$  and have

$$\Delta = \frac{h}{2t}, \quad \epsilon_g = -\frac{h^2}{4t}. \quad (\text{S22})$$

#### IV. FINITE TEMPERATURE EFFECT

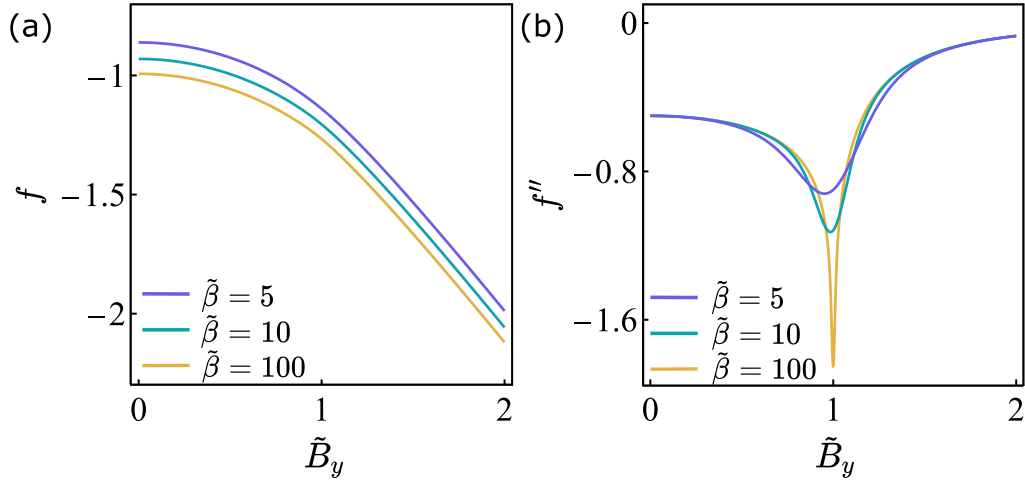

FIG. S4. The free energy density,  $f = F/(NJ)$  (see Eq. S25), and its second-order derivative. (a)  $f$  for various temperature  $\tilde{\beta}$ ; and (b),  $f'' = d^2 f / d\tilde{B}_y^2$ . At zero temperature,  $\tilde{\beta} \rightarrow \infty$ .

Next, we discuss the physics at finite temperature. The total free energy, after Jordan-Wigner transformation, can be given by

$$F = \omega\alpha^2 - \frac{NJ}{2\pi} \int_{-\pi}^{\pi} dk \frac{1}{\tilde{\beta}} \ln 2 \cosh(\tilde{\beta}\Omega_k), \quad \Omega_k = \sqrt{(\tilde{h} - \cos k)^2 + \sin^2 k}, \quad (\text{S23})$$

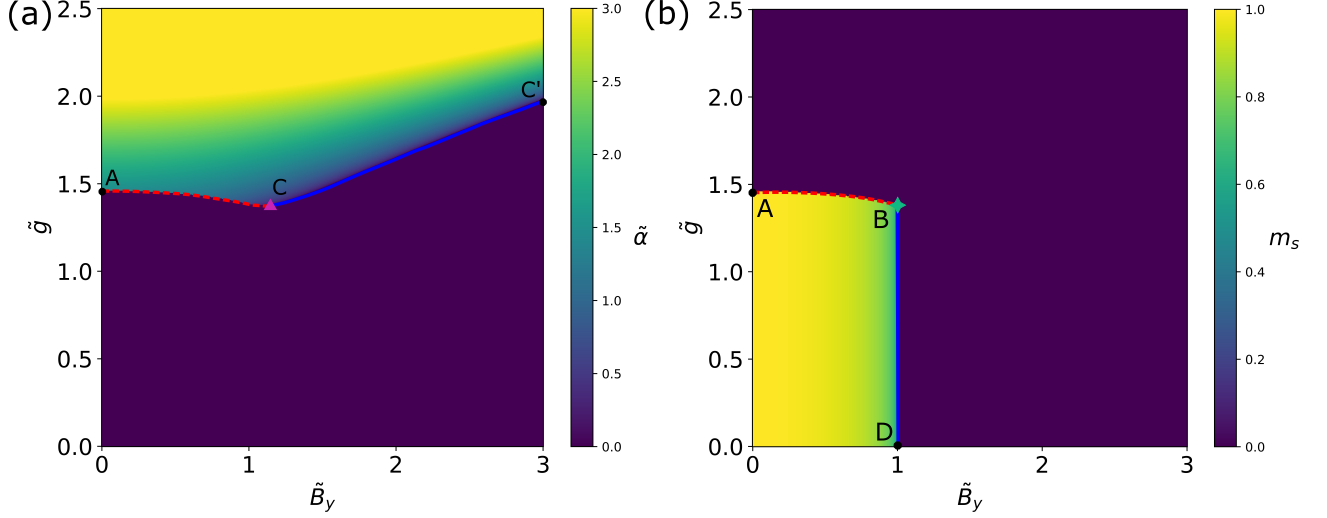

FIG. S5. Phase diagram and order parameters. A, B, C, C', and D have the same meaning as Fig. 1(a) in the main text. The red dashed and blue solid lines denote first- and second-order phase transitions. (a) The superradiant to normal phase diagram. (b) The antiferromagnetic to paramagnetic phase diagram.

where  $\tilde{h} = \sqrt{\tilde{B}_y^2 + \tilde{\alpha}^2}$  as defined in the main text. The energy density is dimensionless as defined in the main text ( $\epsilon_g = \pi E_g / (2JN)$ ), let us define  $\tilde{\beta} = \frac{J}{k_B T} = J\beta$ , which is a dimensionless parameter, then the free energy defined as  $f = F / (NJ)$  will lead to

$$f = \tilde{\gamma} \tilde{\alpha}^2 - \frac{1}{2\pi} \int_{-\pi}^{\pi} dk \frac{1}{\tilde{\beta}} \ln 2 \cosh(\tilde{\beta} \Omega_k), \quad (\text{S24})$$

with  $\tilde{\gamma} = \frac{J\omega}{4g^2}$ ,  $\tilde{\alpha} = \frac{2g\alpha}{\sqrt{NJ}}$ . In the main text, we have defined  $\tilde{g} = \frac{2\sqrt{2}g}{\sqrt{J\pi\omega}}$ , then we have  $\frac{\pi}{2}\tilde{\gamma} = \frac{1}{\tilde{g}^2}$ .

When  $\alpha = 0$ , this model is reduced to the transverse Ising model [12, 13] with free energy density as follows

$$f = -\frac{1}{2\pi} \int_{-\pi}^{\pi} dk \frac{1}{\tilde{\beta}} \ln 2 \cosh(\tilde{\beta} \Omega_k), \quad (\text{S25})$$

which is a function of  $\tilde{B}_y$  and  $\tilde{\beta}$ . The numerical results for this function is presented in Fig. S4 (a), and the second order derivative of  $f$  with respect to temperature,  $f'' = d^2 f / d\tilde{B}_y^2$ , is presented in Fig. S4 (b), which will become singular only at zero temperature. This corresponds to the physics of quantum phase transition, which is the phase transition from antiferromagnetic to paramagnetic phase of the quantum Ising model. At finite temperature, it will become a smooth crossover process. Thus, at finite temperature, the unilateral critical endpoint will not be well defined anymore, and the essential physics should be the transition from the normal phase to the superradiant phase, in which the tricritical point separating the first- and second-order phase transition will become most relevant.

The values of  $\tilde{B}_y^C, \tilde{g}^C$  for the tricritical point at finite temperature can be obtained from

$$\left. \frac{\partial f}{\partial \tilde{h}} \right|_{\tilde{h}=\tilde{B}_y^C} = 0, \quad \left. \frac{\partial^2 f}{\partial \tilde{h}^2} \right|_{\tilde{h}=\tilde{B}_y^C} = 0. \quad (\text{S26})$$

It gives the boundary of the first- and second-order phase transitions, corresponding to the purple line in the main text Fig. 4(c). From this result, it is expected that at high temperatures, only the second-order phase transition is allowed. This diagram consists of two regimes. In the red regime, the transition from the normal phase to the superradiant phase by increasing coupling  $g$  is first-order, and in the blue regime, the transition is second-order. When  $\tilde{B}_y = 0$ , at the dome of the red regime in the main text Fig. 3(c), the blue point along the vertical axis means that when  $T > T_c$ , only the second-order transition is allowed. The critical temperature  $T_c$  and  $\tilde{g}$  of the red point are obtained by

$$\left. \frac{\partial f}{\partial \tilde{h}} \right|_{\tilde{h}=0} = 0, \quad \left. \frac{\partial^2 f}{\partial \tilde{h}^2} \right|_{\tilde{h}=0} = 0, \quad (\text{S27})$$

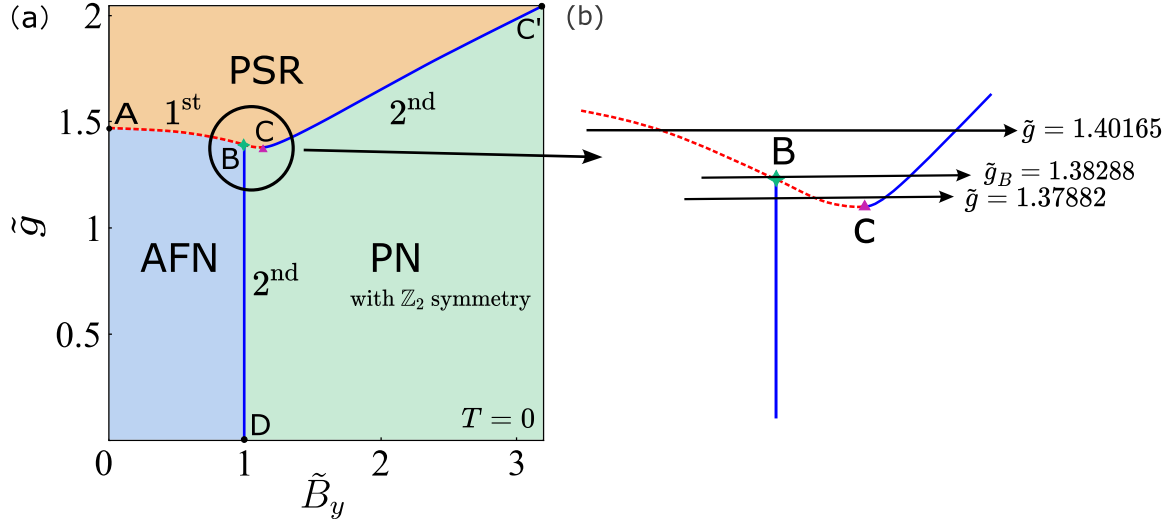

FIG. S6. (a) Phase diagram, which is the same as Fig. 1(a) in the main text. (b) Three horizon lines for fixed  $\tilde{g} = 1.40165$ ,  $1.38288$ , and  $1.37882$ , which are considered in Fig. S7. The red dashed line means a first-order phase transition, and the blue solid lines mean second-order phase transitions.

because at the dome point,  $\tilde{B}_y^C = 0$ . By solving the above equations using numerical methods, we can obtain  $\tilde{\beta}^* = 1.14299$ , with  $k_B T_c = J/\tilde{\beta}^*$ , and  $\tilde{g} = 1.45865$ . Moreover, with the numerical calculation, we find

$$f = -0.478284 + 0.004487\tilde{\alpha}^6 + \dots, \quad (\text{S28})$$

which is still a tricritical point dominated by the  $\tilde{\alpha}^6$  term.

## V. UNILATERAL CRITICAL ENDPOINT

We supplement details about the two order parameters  $\tilde{\alpha}$  and  $m_s$ , as defined above. According to Ref. [14], we can obtain the exact expression of the  $m_s$

$$\begin{aligned} m_s &= (1 - \tilde{h}^2)^{1/8}, \quad 0 \leq \tilde{h} < 1; \\ m_s &= 0, \quad \tilde{h} > 1, \end{aligned} \quad (\text{S29})$$

with  $\tilde{h} = \sqrt{\tilde{B}_y^2 + \tilde{\alpha}^2}$ , thus  $\tilde{h} \geq \tilde{B}_y$ . The order parameters can be determined by minimizing the ground state energy. In Fig. S5, we plot the phase diagram (corresponding to Fig. 1(a) in the main text) in terms of these two order parameters, from which one can have an explicit view of the special critical points and the first- and second-order phase transitions.

Since the unilateral critical endpoint is the most important in this work, finally, let us focus on the critical behavior of the UCEP, i.e., point B in Fig. 1(a) in the main text. We consider the evolution in three horizontal lines, as shown in Fig. S6. We fix  $\tilde{g} \sim \tilde{g}_B = 1.38288$ , and change  $\tilde{B}_y$  from  $\tilde{B}_y < 1$  to  $\tilde{B}_y > 1$  to calculate the critical behavior of the UCEP. We find that, when  $\tilde{g}$  is slightly larger than  $\tilde{g}_B$  (see Fig. S7 (a) and (b), corresponding to the horizontal line in Fig. S6 (b) with  $\tilde{g} = 1.40165$ ), the order parameters  $m_s$  and  $\tilde{\alpha}$  will simultaneously undergo a first order transition from AFN to PSR, corresponding to line AB in Fig. 1(a). From Fig. S7 (c) and (d) (corresponding to the horizontal line in Fig. S6 (b) with  $\tilde{g} = \tilde{g}_B = 1.38288$ ), the two order parameters will undergo the second and first-order phase transitions simultaneously at the UCEP. The order parameter  $m_s$  exhibits the same critical behavior as the antiferromagnetic-to-paramagnetic transition in the transverse-field Ising model [14] when  $\tilde{B}_y \rightarrow 1^-$ , and the same applies along the BD line in the main text Fig. 1 (a) of both sides  $\tilde{B}_y \rightarrow 1^\pm$ . When  $\tilde{g}$  is a bit smaller than  $\tilde{g}_B$  (see Fig. S7 (e) and (f), corresponding to the red horizontal line in Fig. S6 (b) with  $\tilde{g} = 1.37882$ ), the first-order and second-order phase transitions of the two order parameters split apart and occur at different points, corresponding to line BC and BD in Fig. 1(a). Above all, two order parameters will undergo two different phase transitions at the UCEP.

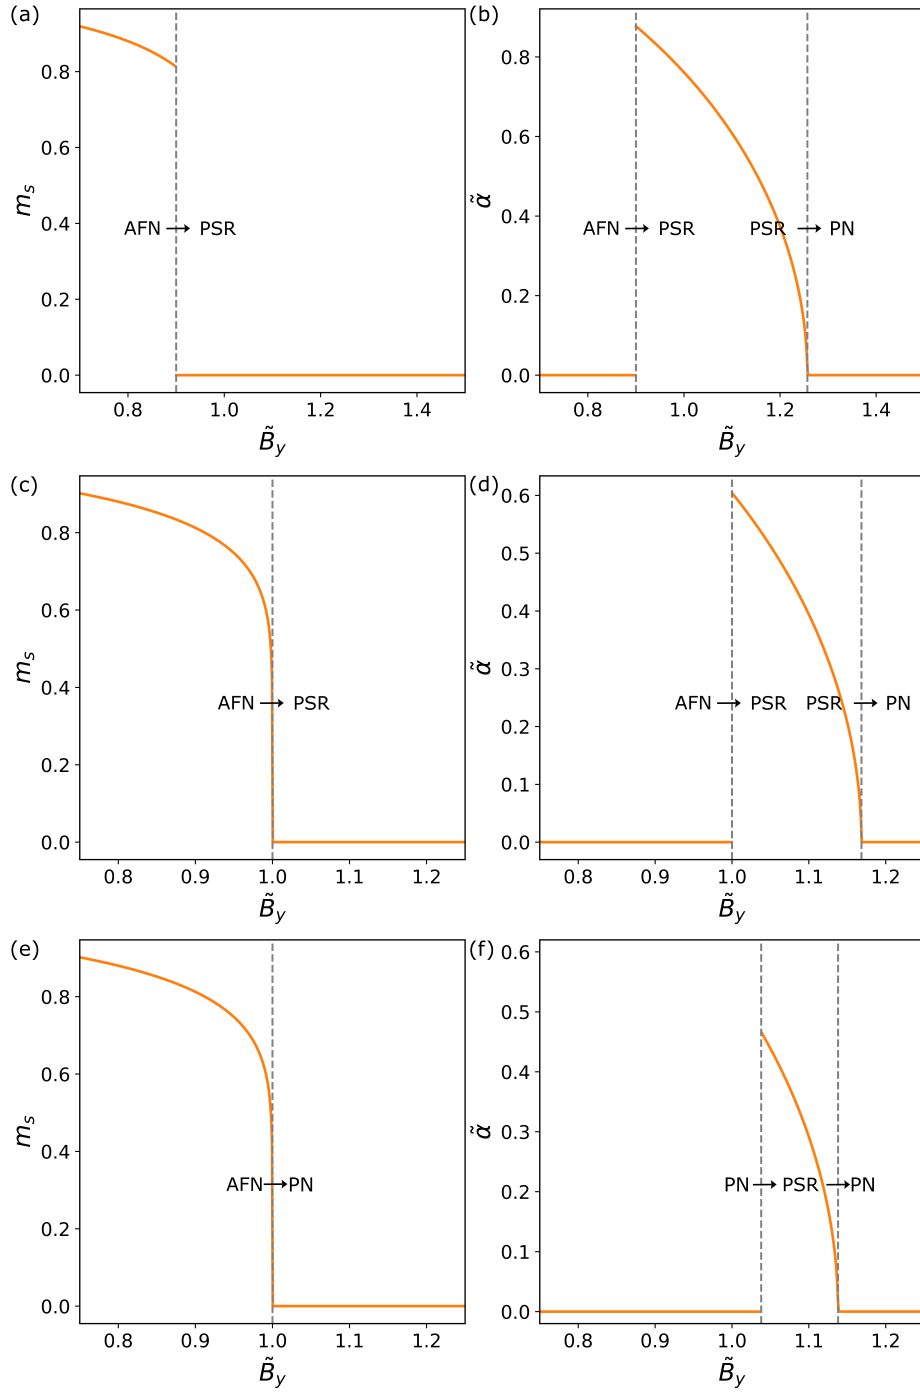

FIG. S7. Evolution of the two order parameters as a function of  $\tilde{B}_y$  near the critical endpoint. (a) and (b),  $\tilde{g} = 1.40165 > \tilde{g}_B$ . The first-order transition occurs at  $\tilde{B}_y = 0.9$  for both  $m_s$  and  $\tilde{\alpha}$  and the second-order phase transition at  $\tilde{B}_y = 1.25854$  in (b) for  $\tilde{\alpha}$ . (c) and (d),  $\tilde{g} = \tilde{g}_B = 1.38288$ . The two order parameters  $m_s$  and  $\tilde{\alpha}$  simultaneously undergo second- and first-order phase transitions, respectively, at the same point ( $\tilde{B}_y = 1$ ); the second-order transition in (d) is at  $\tilde{B}_y = 1.16845$ . (e) and (f),  $\tilde{g} = 1.37882 < \tilde{g}_B$ . The phase transition of  $m_s$  remains a first-order transition at  $\tilde{B}_y = 1$ . The first-order phase transition in (f) is at  $\tilde{B}_y = 1.03801$  and the second-order transition at  $\tilde{B}_y = 1.13626$ . The three phases, AFN, PSR, and PN, are marked in each figure.



This UCEP exhibits unprecedented properties that distinguish it from previously documented critical endpoints and have not been reported in the phase transition literature. We need to employ additional physical probes, such as susceptibility and entanglement entropy, to characterize the unique critical behavior of the UCEP. For the standard Ising model in a transverse field (with  $J = 1$ ):

$$\mathcal{H} = \sum_i \sigma_i^z \sigma_{i+1}^z + h \sigma_i^x, \quad (\text{S30})$$

the transverse magnetic susceptibility can be defined as  $\chi_\perp = \frac{\partial m_x}{\partial h}$ , where  $m_x = \frac{1}{N} \sum_i \langle \sigma_i^x \rangle$ . And it gives

$$\chi_\perp = -\frac{\partial^2 \epsilon_g}{\partial h^2}, \quad (\text{S31})$$

where  $\epsilon_g$  is the ground state energy density [15, 16]. With the analytic expression of  $\epsilon_g$  mentioned in the main text [13, 16]

$$\epsilon_g = -|h-1|E\left(-\frac{4h}{(h-1)^2}\right), \quad (\text{S32})$$

we can get the expression of  $\chi_\perp$

$$\chi_\perp = \frac{-(h-1)^2 E\left(-\frac{4h}{(h-1)^2}\right) + (1+h^2)K\left(-\frac{4h}{(h-1)^2}\right)}{2|h-1|h^2}, \quad (\text{S33})$$

where  $K(\dots)$  denotes complete elliptic integral of the first kind. The  $\chi_\perp(h)$  is shown in the Fig. S8 (a).

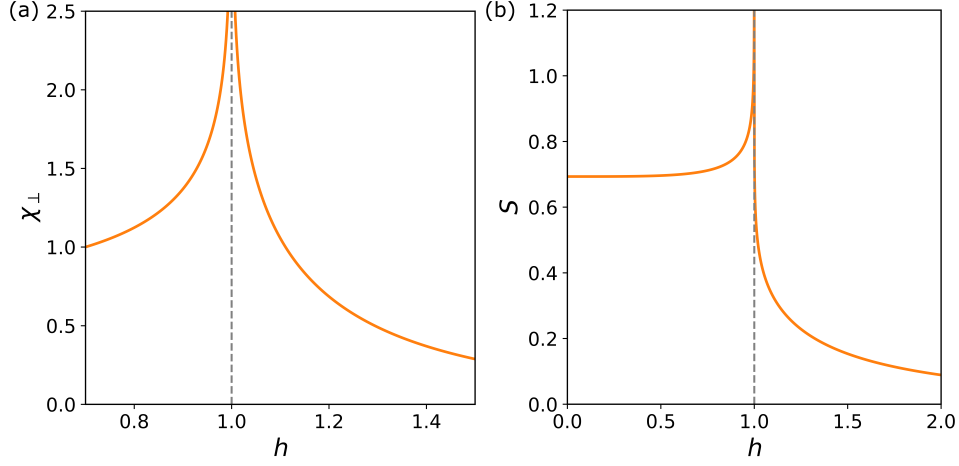

FIG. S8. (a) The transverse magnetic susceptibility of the 1D transverse field Ising model [15, 16]. (b) The entanglement entropy of the 1D transverse field Ising model [16, 17].

We consider the critical behavior of the  $\chi_\perp$  at  $h = 1$ , and we find (by expand  $\chi_\perp$  at  $h = 1$ ) as  $h \rightarrow 1$

$$\chi_\perp = -1 + \frac{3}{2} \ln 2 - \frac{1}{2} \ln |h-1|. \quad (\text{S34})$$

So the transverse magnetic susceptibility diverges logarithmically at  $h = 1$ , indicating a second-order phase transition as is well-known [13, 15, 16].

Besides, we can use the entanglement entropy as a probe of the phase transition [16, 17]. We can split the spin chain into two half-infinite parts, named A and B. The reduced density matrix of the subsystem A is defined as  $\rho_A = \text{Tr}_B \rho$ , where we assume that the system is in a pure quantum state  $|\Psi\rangle$  and the density matrix of the whole system  $\rho = |\Psi\rangle\langle\Psi|$ . The entanglement entropy can be calculated by

$$S = -\text{Tr} \rho_A \ln \rho_A, \quad (\text{S35})$$

and the entanglement entropy of the transverse Ising model is (with  $\lambda = h^{-1}$ ), for  $\lambda < 1$

$$S = \epsilon \sum_{j=0}^{\infty} \frac{2j+1}{1 + e^{(2j+1)\epsilon}} + \sum_{j=0}^{\infty} \ln(1 + e^{-(2j+1)\epsilon}), \quad (\text{S36})$$

with

$$\epsilon = \pi \frac{K(\sqrt{1-k^2})}{K(k)}, \quad (\text{S37})$$

and  $k = \min[\lambda, \lambda^{-1}]$ . While for  $\lambda > 1$

$$S = \epsilon \sum_{j=0}^{\infty} \frac{2j}{1 + e^{2j\epsilon}} + \sum_{j=0}^{\infty} \ln(1 + e^{-2j\epsilon}). \quad (\text{S38})$$

The plot of entanglement entropy as a function of  $h$  is shown in Fig. S8. It exhibits a divergence at the critical point  $h = 1$ . The critical behavior of entanglement entropy at  $h = 1$  ( $h \rightarrow 1, \lambda \rightarrow 1, \epsilon \rightarrow 0$ ) is [17]

$$S = -\frac{1}{12} \ln |h - 1|. \quad (\text{S39})$$

It exhibits a logarithmic divergence at the critical point  $h = 1$ .

Let us calculate the transverse magnetic susceptibility and the entanglement entropy of our model

$$H = \omega \hat{a}^\dagger \hat{a} + \sum_i J \sigma_i^z \sigma_{i+1}^z + \frac{g}{\sqrt{N}} (\hat{a} + \hat{a}^\dagger) \sigma_i^x + B_y \sigma_i^y. \quad (\text{S40})$$

With the approximation of  $\hat{a} \rightarrow \alpha$  and the rotation (see the main text), the Hamiltonian can be written as

$$\mathcal{H} = \omega \alpha^2 + \sum_i \left[ J \sigma_i^z \sigma_{i+1}^z + \sqrt{\frac{4\alpha^2 g^2}{N} + B_y^2} \sigma_i^x \right]. \quad (\text{S41})$$

The spin part of the above Hamiltonian is a transverse field Ising model (see Eq. S30), the equivalent magnetic field is  $\tilde{h} = \sqrt{\tilde{B}_y^2 + \tilde{\alpha}^2}$  with  $\tilde{\alpha}^2 = \frac{4\alpha^2 g^2}{N J^2}$  as defined in the main text. Before the specific calculation, we need to explain the validity of the results after  $\hat{a} \rightarrow \alpha$ . Firstly, we mainly focus on the critical behaviors in the region near the unilateral critical endpoint, i.e., point B in Fig. 1 (a) in the main text. Point B is located on the line A-B-C, which is the first-order phase transition of the cavity field. This means that the fluctuations of  $\hat{a}$  do not exhibit critical divergence in the thermodynamic limit. Besides, in the superradiant phase, the fluctuation will be suppressed, while in the normal phase, the cavity mode is gapped and  $\langle \hat{a} \rangle = 0$ , so the fluctuation will not take the dominant position. In the normal phase, the cavity-field fluctuations only renormalize spin parameters by finite amounts, without altering the spin universality class [18–20]. Furthermore,  $\hat{a} \rightarrow \alpha$  is equivalent to the saddle approximation in the main text, and as discussed in the main text, it is an exact result [21].

Let  $\boldsymbol{\sigma}_i = (\sigma_i^x, \sigma_i^y, \sigma_i^z)$  and  $\hat{\mathbf{n}}_\perp = (\tilde{\alpha}, \tilde{B}_y, 0)/\sqrt{\tilde{B}_y^2 + \tilde{\alpha}^2}$ . Then we can define  $\sigma_i^\perp = \boldsymbol{\sigma}_i \cdot \hat{\mathbf{n}}_\perp$ , and the transverse magnetic susceptibility  $m_\perp = \frac{1}{N} \sum_i \langle \sigma_i^\perp \rangle$ . After rotation, the spin operator  $\sigma_i^\perp$  becomes the  $\sigma_i^x$  in the Eq. S41. Then we define

$$\chi_\perp \equiv \frac{\partial m_\perp}{\partial \tilde{h}}. \quad (\text{S42})$$

The above partial derivative is calculated when  $\tilde{g}$  is fixed.  $\chi_\perp$  measures how the transverse spin polarization changes when the field is slightly varied along the effective transverse axis  $\hat{\mathbf{n}}_\perp$ . In the rotated frame, this coincides with the standard transverse field Ising susceptibility. In the superradiant phase, with a fixed  $\tilde{g}$ , the self-consistent  $\tilde{h}$  is fixed and does not vary with  $\tilde{B}_y$ . Therefore  $\chi_\perp$ , with respect to  $\tilde{B}_y$ , is constant. While in the normal phase,  $\tilde{\alpha} = 0$ ,  $\tilde{h} = \tilde{B}_y$ ,  $\chi_\perp$  reduces to the magnetic susceptibility of the transverse field Ising model with transverse field  $\tilde{h} = \tilde{B}_y$ . After  $\hat{a} \rightarrow \alpha$ , the entanglement entropy can be defined as that in the transverse field Ising model. With  $\tilde{g}$  fixed, it also remains unchanged throughout the superradiant phase. In the normal phase, the entanglement entropy reduces to that of the transverse-field Ising model.

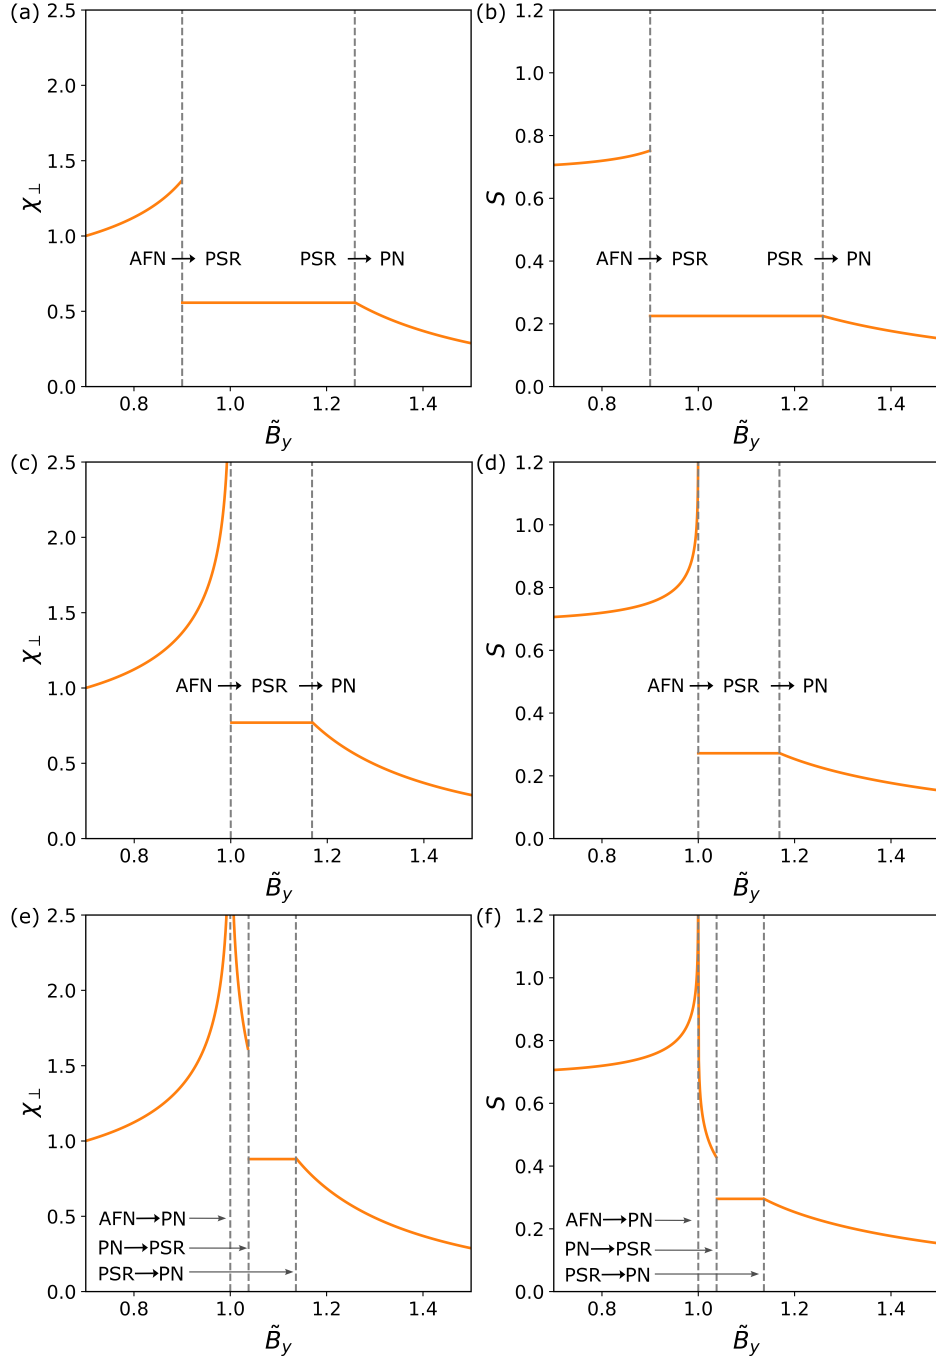

FIG. S9. Evolution of the transverse magnetic susceptibility and entanglement entropy of the spin system as a function of  $\tilde{B}_y$  near the UCEP. (a) and (b),  $\tilde{g} = 1.40165 > \tilde{g}_B$ . The first-order transition occurs at  $\tilde{B}_y = 0.9$ , exhibited by both  $\chi_\perp$  and  $\tilde{\alpha}$  and the second-order phase transition at  $\tilde{B}_y = 1.25854$ . (c) and (d),  $\tilde{g} = \tilde{g}_B = 1.38288$ . When  $\tilde{B}_y \rightarrow 1^-$ ,  $\chi_\perp$  and  $S$  logarithmically diverge, while when  $\tilde{B}_y \rightarrow 1^+$   $\chi_\perp$  and  $S$  remain finite. The second-order phase transition is at  $\tilde{B}_y = 1.16845$ . (e) and (f),  $\tilde{g} = 1.37882 < \tilde{g}_B$ . The system undergoes an Ising-type phase transition (second-order) at  $\tilde{B}_y = 1$ . The first-order phase transition is at  $\tilde{B}_y = 1.03801$ , and the second-order transition at  $\tilde{B}_y = 1.13626$ . The three phases, AFN, PSR, and PN, are marked in each figure.

In Fig. S7, we show how the two order parameters vary with  $\tilde{B}_y$  as  $\tilde{g}$  is fixed (corresponding to Fig. S6). We now discuss the transverse susceptibility and the entanglement entropy of the spin system, exhibiting an unprecedented one-sided critical behavior. In Fig. S9 (a) and (b), when  $\tilde{g}$  is slightly larger than  $\tilde{g}_B$ , both  $\chi_\perp$  and  $S$  have a finite jump at  $\tilde{B}_y = 0.9$ , corresponding to a first-order phase transition from AFN to PSR; and a derivative discontinuity at  $\tilde{B}_y = 1.25854$ , resulted from the second-order phase transition from PSR to PN. In Fig. S9 (e) and (f),  $\chi_\perp$  and  $S$  indicate that the system firstly undergoes an Ising-type transition, followed by first- and second-order superradiant transitions.

The intriguing critical behavior at the UCEP is depicted in Fig. S9 (c) and (d). When  $\tilde{B} \rightarrow 1^-$ ,  $\chi_\perp \sim -\frac{1}{2} \ln |\tilde{B}_y - 1|$  and  $S \sim -\frac{1}{12} \ln |\tilde{B}_y - 1|$ , logarithmically diverge; while when  $\tilde{B}_y \rightarrow 1^+$ , both  $\chi_\perp$  and  $S$  remain a finite value and will not diverge as the left side. These results are consistent with the order parameters. In the Fig. S7. (c) and (d),  $m_s$  exhibits a corresponding phase transition when  $\tilde{B}_y \rightarrow 1^-$  with  $\tilde{\alpha}$  remains 0; for the right side,  $\tilde{\alpha}$  gives a discontinuous jump while  $m_s = 0$ .

All of the above evidence points to that, at point B in the main text Fig. 1 (a), the system has a unilateral critical behavior. When approaching the critical endpoint from the AFN side, the critical behavior is Ising-type, with  $\chi_\perp$  and  $S$  diverging, while approaching this point from the other side, the critical behavior is totally different, similar to a first-order phase transition. Therefore, we designate this point as the unilateral critical endpoint.

In the standard Landau framework, the free energy is assumed to be an analytic expansion of the order parameters. Consequently, the singular behavior near criticality is governed by a single analytic form, yielding the same critical exponents on both sides of the transition (differences may appear only as amplitude ratios) [22, 23]. Next, we explore the general form of the free energy for the unilateral critical endpoint. We set the following form of the density of the free energy:

$$f = c_1(\tilde{\alpha}^2 + c_2) + (\tilde{\alpha}^2 + c_2)^2 \ln |\tilde{\alpha}^2 + c_2|, \quad (\text{S43})$$

where  $c_1$  and  $c_2$  are parameters. Only one of the coefficients of  $\tilde{\alpha}^2$  and  $\tilde{\alpha}^4 \ln \tilde{\alpha}^2$  is necessary. For zero temperature, the above density of the free energy becomes the density of the ground state energy. From the main text, the expansion of the ground state energy at the critical endpoint gives

$$\epsilon_g = \frac{1 - 2\tilde{g}^2}{\tilde{g}^2} + \frac{2 - \tilde{g}^2}{2\tilde{g}^2} \tilde{\alpha}^2 + \frac{1}{16} \ln(\tilde{\alpha}^2) \tilde{\alpha}^4 \quad (\text{S44})$$

With  $\tilde{g}_B = 1.38288$ , we have

$$\epsilon_g = -1.477 + 0.023\tilde{\alpha}^2 + 0.0625 \log(\tilde{\alpha}^2) \tilde{\alpha}^4. \quad (\text{S45})$$

We care about the critical behavior around  $\tilde{B}_y = 1$  with a fixed  $\tilde{g}$ . At the critical endpoint,  $\tilde{h} = \sqrt{(\tilde{B}_y + \delta\tilde{B}_y)^2 + \tilde{\alpha}^2}$ , the expansion gives (when  $\tilde{B}_y = 1$ )

$$\tilde{h} - 1 = \delta\tilde{B}_y + \frac{1}{2}\tilde{\alpha}^2 = \frac{1}{2}(\tilde{\alpha}^2 + 2\delta\tilde{B}_y). \quad (\text{S46})$$

Then it leads to

$$\epsilon_g = \frac{1 - 2\tilde{g}^2}{\tilde{g}^2} + \frac{2 - \tilde{g}^2}{2\tilde{g}^2}(\tilde{\alpha}^2 + 2\delta\tilde{B}_y) + \frac{1}{16} \ln(|\tilde{\alpha}^2 + 2\delta\tilde{B}_y|)(\tilde{\alpha}^2 + 2\delta\tilde{B}_y)^2. \quad (\text{S47})$$

The constant term can be ignored. We have

$$\epsilon_g = \frac{2 - \tilde{g}^2}{2\tilde{g}^2}(\tilde{\alpha}^2 + 2\delta\tilde{B}_y) + \frac{1}{16} \ln(|\tilde{\alpha}^2 + 2\delta\tilde{B}_y|)(\tilde{\alpha}^2 + 2\delta\tilde{B}_y)^2. \quad (\text{S48})$$

Let us compare Eq. S43 and Eq. S44, and we have

$$c_1 = \frac{8(2 - \tilde{g}^2)}{\tilde{g}^2}, \quad c_2 = 2\delta\tilde{B}_y; \quad (\text{S49})$$

and

$$f = \frac{8(2 - \tilde{g}^2)}{\tilde{g}^2}(\tilde{\alpha}^2 + 2\delta\tilde{B}_y) + (\tilde{\alpha}^2 + 2\delta\tilde{B}_y)^2 \ln(|\tilde{\alpha}^2 + 2\delta\tilde{B}_y|). \quad (\text{S50})$$

Now, let's explain why the free energy Eq. S43 yields the unilateral critical endpoint. Because  $\tilde{h} \sim \tilde{\alpha}^2$ , the susceptibility can be obtained by (when  $c_2 = 0$ )

$$\chi = \frac{\partial^2 f}{\partial \tilde{h}^2} = \frac{\partial^2 f}{\partial (\tilde{\alpha}^2)^2} = 3 + 2 \ln \tilde{\alpha}^2. \quad (\text{S51})$$

So  $\chi$  logarithmically diverges at  $\tilde{\alpha} \rightarrow 0$ .  $c_2$  shifts the graph of the function along the  $\tilde{\alpha}^2$ -axis. The critical case is depicted in Fig. S10 (a) with  $c_1$  fixed. For  $c_2 = 0$ , both of the two local minima of the blue-green line give  $f = 0$ . The black dots represent non-analytic points. So, when  $c_2 \rightarrow 0^-$ ,  $\tilde{\alpha} = 0$ , corresponding to the yellow dashed line,  $\chi$  approaches logarithmic divergence; while for  $c_2 \rightarrow 0^+$ ,  $\alpha \neq 0$ , corresponding to the purple dashed line,  $\chi$  does not diverge. Therefore, it exhibits the unilateral critical behavior.

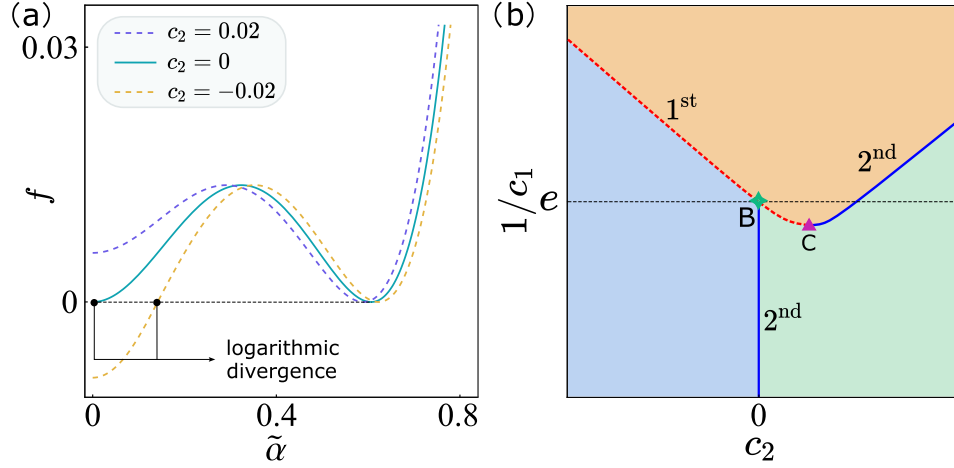

FIG. S10. (a) The free energy exhibits in Eq. S43 with  $c_1 = 1/e$ . The black dots represent non-analytic points. (b) The phase diagram resulted from Eq. S43. The red dashed and blue solid lines represent first- and second-order phase transitions. B is the unilateral critical endpoint, and C is the tricritical point.

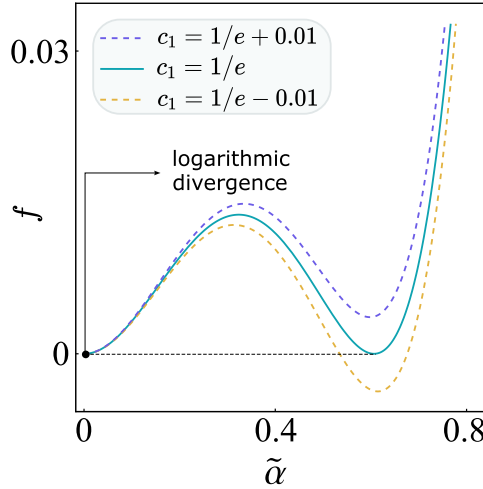

FIG. S11. (a) The free energy exhibits in Eq. S43 with  $c_2 = 0$ .

Now, let us discuss why the schematic phase diagram exhibited in Fig. S10 (b) results from the free energy Eq. S43. When  $c_1 = \frac{1}{e}$ , both of the two local minima of the blue-green line in Fig. S10 (a) give  $f = 0$ , which represents the one-sided critical behavior. If  $c_1$  increases ( $1/c_1$  decreases), corresponding to the purple dashed line in the Fig. S11, the free energy of the two local minima splits and the local minimum at  $\tilde{\alpha} \neq 0$  is lifted. So if we change  $c_2$ , the system will first undergo a continuous phase transition (the blue solid vertical line connecting point B depicted in the Fig. S10 (b)), and followed by a first-order phase transition (the red dashed line BC in the Fig. S10(b)). When

$c_2$  crosses the local minimum at  $\tilde{\alpha} \neq 0$ , the system undergoes a second-order phase transition. If  $c_1$  continues to decrease, the local minimum at  $\tilde{\alpha} \neq 0$  will shrink and finally disappear, rendering the tricritical point (point C).

Furthermore, we give the analytic results. For the unilateral critical endpoint, two local minima are equal. It leads to

$$f(\tilde{\alpha}) = 0, \quad c_2 = 0, \quad \frac{\partial f}{\partial \tilde{\alpha}} = 0. \quad (\text{S52})$$

When  $c_2 = 0$ ,  $f(\tilde{\alpha}) = 0$  leads to,

$$c_1 \tilde{\alpha}^2 + \tilde{\alpha}^4 \ln \tilde{\alpha}^2 = 0; \quad (\text{S53})$$

and

$$\frac{\partial f}{\partial \tilde{\alpha}} = 2c_1 \tilde{\alpha} + 2\tilde{\alpha}^3 + 4\tilde{\alpha}^3 \ln \tilde{\alpha}^2 = 0. \quad (\text{S54})$$

From the above analysis, we have

$$c_1 = \frac{1}{e}, \quad c_2 = 0, \quad \tilde{\alpha} = \frac{1}{\sqrt{e}}, \quad (\text{S55})$$

at the unilateral critical endpoint, and  $e$  is Euler's number. With  $c_1 = \frac{8(2-\tilde{g}^2)}{\tilde{g}^2}$ , then the  $\tilde{g}$  of the unilateral critical endpoint is obtained by

$$\tilde{g} = 4\sqrt{\frac{e}{1+8e}} \approx 1.38278. \quad (\text{S56})$$

Compared to the result in the main text,  $\tilde{g}_B = 1.38288$ , Eq. S56 is accurate, and a tiny deviation resulted from the assumption  $\tilde{\alpha} \ll 1$ . Besides, for the tricritical point, we have

$$\frac{\partial f}{\partial \tilde{\alpha}} = 0, \quad \frac{\partial^2 f}{\partial \tilde{\alpha}^2} = 0. \quad (\text{S57})$$

It leads to

$$\frac{\partial f}{\partial \tilde{\alpha}} = 2c_1 \tilde{\alpha} + 2\tilde{\alpha}^3 + 4\tilde{\alpha}^3 \ln \tilde{\alpha}^2 = 0, \quad (\text{S58})$$

and

$$\frac{\partial^2 f}{\partial \tilde{\alpha}^2} = 2c_1 + 14\tilde{\alpha}^2 + 12\tilde{\alpha}^2 \ln \tilde{\alpha}^2 = 0. \quad (\text{S59})$$

We can obtain

$$c_1 = \frac{2}{e^{3/2}}, \quad c_2 = \frac{1}{e^{3/2}}. \quad (\text{S60})$$

It gives  $\tilde{g} = 2e^{3/4} \sqrt{\frac{2}{1+4e^{3/2}}} \approx 1.37635$ , and  $\tilde{B}_y = 1 + \delta \tilde{B}_y = 1 + \frac{1}{2e^{3/2}} = 1.11157$ , for the tricritical point, compared to the  $\tilde{g}_C = 1.37698$  and  $\tilde{B}_y^C = 1.10022$  in the main text.

In summary, we derive the unilateral criticality and give the minimal universal description of it with a logarithmic singularity in Eq. S43, which yields a unilateral critical endpoint (at  $c_1 = \frac{1}{e}, c_2 = 0$ ) and a tricritical point (at  $c_1 = \frac{2}{e^{3/2}}, c_2 = \frac{1}{e^{3/2}}$ ), depicted in Fig. S10 (b). There are many other models that may have a similar logarithmically singular form  $f \sim \tilde{h}^2 \ln |\tilde{h}|$  [24, 25], such as the two-dimensional classical Ising model [26], long-range Ising models at the Sak boundary [27, 28], relativistic 1+1-dimensional Dirac theories and the Gross-Neveu model [29], and anisotropic Lifshitz  $O(N)$  models at the upper critical dimension  $d_{\text{eff}} = d + z = 4$  [30–32]. With coupling to a non-local operator [18, 33],  $\tilde{h} \sim c_2 + \tilde{\alpha}^2$ , the unilateral critical endpoint and the attendant tricritical point could happen. Thus, the unilateral criticality is not a model-specific peculiarity, representing a new, potentially universal type of phase transition, likely realized in a broad class of systems.

---

[1] Andrea Morales, Philip Zupancic, Julian Léonard, Tilman Esslinger, and Tobias Donner, “Coupling two order parameters in a quantum gas,” *Nature materials* **17**, 686–690 (2018).

- [2] T. S. Chang, Alex Hankey, and H. Eugene Stanley, “Generalized scaling hypothesis in multicomponent systems. i. classification of critical points by order and scaling at tricritical points,” *Phys. Rev. B* **8**, 346–364 (1973).
- [3] Alex Hankey, H. Eugene Stanley, and T. S. Chang, “Geometric predictions of scaling at tricritical points,” *Phys. Rev. Lett.* **29**, 278–281 (1972).
- [4] Robert B. Griffiths, “Phase diagrams and higher-order critical points,” *Phys. Rev. B* **12**, 345–355 (1975).
- [5] G. F. Tuthill, J. F. Nicoll, and H. E. Stanley, “Renormalization-group calculation of the critical-point exponent  $\eta$  for a critical point of arbitrary order,” *Phys. Rev. B* **11**, 4579–4582 (1975).
- [6] Eberhard K. Riedel, “Scaling approach to tricritical phase transitions,” *Phys. Rev. Lett.* **28**, 675–678 (1972).
- [7] T.S Chang, D.D Vvedensky, and J.F Nicoll, “Differential renormalization-group generators for static and dynamic critical phenomena,” *Phys. Rep.* **217**, 279–360 (1992).
- [8] Robert B. Griffiths, “Thermodynamics near the two-fluid critical mixing point in  $\text{He}^3$  -  $\text{He}^4$ ,” *Phys. Rev. Lett.* **24**, 715–717 (1970).
- [9] M. Soriente, T. Donner, R. Chitra, and O. Zilberberg, “Dissipation-induced anomalous multicritical phenomena,” *Phys. Rev. Lett.* **120**, 183603 (2018).
- [10] O. Castaños, E. Nahmad-Achar, R. López-Peña, and J. G. Hirsch, “Universal critical behavior in the Dicke model,” *Phys. Rev. A* **86**, 023814 (2012).
- [11] Vincent R. Overbeck, Mohammad F. Maghrebi, Alexey V. Gorshkov, and Hendrik Weimer, “Multicritical behavior in dissipative Ising models,” *Phys. Rev. A* **95**, 042133 (2017).
- [12] John B Parkinson and Damian JJ Farnell, *An introduction to quantum spin systems*, Vol. 816 (Springer, 2010).
- [13] Fabio Franchini *et al.*, *An introduction to integrable techniques for one-dimensional quantum systems*, Vol. 940 (Springer, 2017).
- [14] Pierre Pfeuty, “The one-dimensional Ising model with a transverse field,” *ANNALS of Physics* **57**, 79–90 (1970).
- [15] R. Jullien, P. Pfeuty, J. N. Fields, and S. Doniach, “Zero-temperature renormalization method for quantum systems. I. Ising model in a transverse field in one dimension,” *Phys. Rev. B* **18**, 3568–3578 (1978).
- [16] Sei Suzuki, Jun-ichi Inoue, and Bikas K Chakrabarti, *Quantum Ising phases and transitions in transverse Ising models*, Vol. 862 (Springer, 2012).
- [17] Pasquale Calabrese and John Cardy, “Entanglement entropy and quantum field theory,” *Journal of statistical mechanics: theory and experiment* **2004**, P06002 (2004).
- [18] Helmut Ritsch, Peter Domokos, Ferdinand Brennecke, and Tilman Esslinger, “Cold atoms in cavity-generated dynamical optical potentials,” *Rev. Mod. Phys.* **85**, 553 (2013).
- [19] Peter Kirton, Mor M. Roses, Jonathan Keeling, and Emanuele G. Dalla Torre, “Introduction to the dicke model: From equilibrium to nonequilibrium, and vice versa,” *Advanced Quantum Technologies* **2**, 1800043 (2019).
- [20] Fran çois Damanet, Andrew J. Daley, and Jonathan Keeling, “Atom-only descriptions of the driven-dissipative Dicke model,” *Phys. Rev. A* **99**, 033845 (2019).
- [21] Wei-Feng Zhuang, Bin Geng, Hong-Gang Luo, Guang-Can Guo, and Ming Gong, “Universality class and exact phase boundary in the superradiant phase transition,” *Phys. Rev. A* **104**, 053308 (2021).
- [22] Nigel Goldenfeld, *Lectures on phase transitions and the renormalization group* (CRC Press, 2018).
- [23] Subir Sachdev, *Quantum Phase Transitions*, 2nd ed. (Cambridge University Press, 2011).
- [24] Franz J. Wegner, “Corrections to Scaling Laws,” *Phys. Rev. B* **5**, 4529–4536 (1972).
- [25] Franz J. Wegner and Eberhard K. Riedel, “Logarithmic Corrections to the Molecular-Field Behavior of Critical and Tricritical Systems,” *Phys. Rev. B* **7**, 248–256 (1973).
- [26] Franz Wegner, “Two-Dimensional Ising Model,” in *Supermathematics and its Applications in Statistical Physics: Grassmann Variables and the Method of Supersymmetry* (Springer Berlin Heidelberg, Berlin, Heidelberg, 2016) pp. 75–100.
- [27] Nicolò Defenu, Tobias Donner, Tommaso Macrì, Guido Pagano, Stefano Ruffo, and Andrea Trombettoni, “Long-range interacting quantum systems,” *Rev. Mod. Phys.* **95**, 035002 (2023).
- [28] Jan Alexander Koziol, Anja Langheld, Sebastian C. Kapfer, and Kai Phillip Schmidt, “Quantum-critical properties of the long-range transverse-field Ising model from quantum Monte Carlo simulations,” *Phys. Rev. B* **103**, 245135 (2021).
- [29] David J. Gross and André Neveu, “Dynamical symmetry breaking in asymptotically free field theories,” *Phys. Rev. D* **10**, 3235–3253 (1974).
- [30] H W Diehl and M Shpot, “Lifshitz-point critical behaviour to  $O(\epsilon^2)$ ,” *Journal of Physics A: Mathematical and General* **34**, 9101–9105 (2001).
- [31] H. W. Diehl, “Critical Behavior at M-Axial Lifshitz Points,” (2002), arXiv:cond-mat/0205284 [cond-mat.stat-mech].
- [32] C. Mergulhão and C. E. I. Carneiro, “Field-theoretic approach to the Lifshitz point,” *Phys. Rev. B* **58**, 6047–6056 (1998).
- [33] Farokh Mivehvar, Francesco Piazza, Tobias Donner, and Helmut Ritsch, “Cavity QED with quantum gases: new paradigms in many-body physics,” *Advances in Physics* **70**, 1–153 (2021).
